# Supplementary material for: Reducing Human-Robot Goal State Divergence with Environment Design
Source: arXiv:2404.15184 source file (2024-04-10)
Supplement: Supplementary file 1 [file 5-2-supplementary.tex]

\section{Supporting Plan Subsets}
\textcolor{blue}{As previously discussed, the definitions provided in the main portion of this paper are quite relaxed in the plans being considered.}
By considering the space of all plans we are effectively considering a much larger space of models than what would ever be expected by a human or executed by the robot.
This will result in weaker bounds than what might be effective. For the robot plan, one of the most direct considerations we can make is to effectively restrict the space of plans to just the optimal plans. However, to make assertions about the possible human plans, we will need to associate a decision-making model with the human. A popular option that is widely used in human-AI interaction literature is the noisy-rational model, where the likelihood of the human choosing a plan is given as
\[P(\pi) \propto \epsilon^{-\beta \times c(\pi)}\]
Where $\beta$ is a parameter called the rationality parameter. Now we can only consider plans that are above some probability threshold $\epsilon$. For any such probability threshold, there will be a corresponding cost value $C_{\epsilon}$, such that for any plan $\pi$, where $c(\pi) > C_{\epsilon}$, you will have $P(\pi) < \epsilon$. We will denote the corresponding upper and lower bounds of $\GSD$, where the plan spaces are bounded as described above as $\MxGDstr$ and $\MnGDstr$.

We can form variations of Definition 6 provided in the main paper, by replacing $\MxGD$ and $\MnGD$, with $\MxGDstr$ and $\MnGDstr$. 

\subsection{Calculating these new bounds}
To calculate $\MxGDstr$ and $\MnGDstr$, we can place additional constraints on the human part of the plan to restrict plans of cost higher than the cost $C_{\epsilon}$. While in the most general case, this would involve additional book-keeping, one of the special cases, namely restricting to just optimal plans in the human model (represented as  $\MxGDOpt$ and $\MnGDOpt$) allows for a surprisingly simple formulation.
\begin{prop}
    For a given compiled model $\mathcal{M^\lambda}$, let us adopt the following cost function
    \begin{itemize}
        \item Cost of the human and robot action copies follows the ordering in the original models. For human action copies, this means, for any two actions $a_1,a_2 \in \mathcal{A^H}'$,  $C^\lambda(a_1) < C^\lambda(a_2)$, if and only if, $C^\mathcal{H}(a_1^\mathcal{H}) < C^\mathcal{H}(a_2^\mathcal{H})$, where $a_1,a_2 \in \mathcal{A^H}$ are the corresponding human actions. The same ordering constraint holds for $\mathcal{A^{R'}}$ and $\mathcal{A^R}$
        \item Cost of the cheapest human action is higher than the costs of the costliest robot plan, i.e., 
        $min_{a \in \mathcal{A^{H}}'}(C^\lambda(a)) > max_{a \in \mathcal{A^{R'}}}(C^\lambda(a)) \times 2^{|\mathcal{F^R}|}$
        \item 
        Cost of the cheapest robot action is higher than the sum of the costs of all check agreement actions, i.e.
        $min_{a \in \mathcal{A^{R'}}}(C^\lambda(a)) > \sum_{f_i^\mathcal{R} \in \mathcal{F^R}} \mathcal{P}_1$
        
        \item Cost of check agreement action is unit cost (i.e. $\mathcal{P}_2 = 1$) and disagreement is $\mathcal{P}_2 = 0$.
    \end{itemize}
     For the given cost function, let $\pi^\lambda$ be an optimal plan, then $\MxGDOpt(\mathcal{M^R}, \mathcal{M^H}) = |\kappa^-(\pi^\lambda)|$.
\end{prop}
\begin{proof} [Proof Sketch]
    The cost function employed ensures that no optimal plan can contain a suboptimal human plan in it. Among all the solutions where $\mathcal{H}(\pi^{\lambda})$ corresponds to an optimal plan, the cost is dominated by  robot actions. 
    Thus no amount of agreement or disagreement would justify the selection of a suboptimal plan for  $\mathcal{R}(\pi^{\lambda})$. Finally, among the optimal robot and human plans, it selects ones that minimize the use of agreement actions.
\end{proof}

One can also calculate $\MnGDOpt$, by using a cost function that is pretty much the same as the one described above, except now $\mathcal{P}_1 =0$ and $\mathcal{P}_2 > 2^{|\mathcal{F^R}|}$. 

\subsection{Updated Compilation}
We had already provided a compilation in the paper that supports the automatic identification of designs for conditions where $\ell=0$ and the design corresponds to merely initial state updates. Now we will provide a more general formulation that relaxes these two assumptions.

As with the previous formulation, each design now corresponds to a specific model component. Though now the component can be any part of the model other than the goals. Changes to the initial state are treated as before by actions that directly update the initial state before the $design\_completed$ action. For the other model changes, we will again introduce a set of design actions $\mathcal{A^D}'$, that will possibly add a fluent each from the set $\mathcal{D}_\mathbb{U}'$. As with previous design actions, we constrain the applicability of these actions to only before the $design\_completed$ action. \textcolor{red}{Now for each model component that will be influenced by these designs, will be made conditioned on these new design fluents.} Let's say a precondition $p$ is added to action $a$ by a design corresponding to fluent $d_i \in \mathcal{A^D}'$, then the human and robot copies of the action $a^\mathcal{H}$ and $a^\mathcal{R}$ will now contain a precondition $\neg d_i \wedge p^\mathcal{H}$ and  $\neg d_i \wedge p$ respectively. If the design results in a precondition being removed, the precondition becomes $d_i \wedge p^\mathcal{H}$. Similarly, for effects, we can introduce conditional effects, where it is conditioned on design fluents from $\mathcal{D}_\mathbb{U}'$. Now if we keep the rest of the compilation the same, we can support designs that update any part of the model.

The next generalization we talked about was to support non-zero $\ell$. To do this, we will introduce a new set of fluents $\mathcal{F}^\ell$, where $|\mathcal{F}^\ell|=\ell$, is used to track the budget. To ensure that we can only allow $\ell$ possible disagreements, we re-introduce the disagreement actions. Now we will have $|\mathcal{F}|\times\ell$ copies. One for each fluent and will use up one of the possible allotted budgets. \textcolor{red}{To capture this, we will add to the precondition the $i^{th}$ copy of any disagreement action for fluent $f$, the fluent $f^\ell_{i}$ (from the set $\mathcal{F}^\ell$).} The disagreement action will also delete this fluent. So at most $\ell$ disagreement actions can be used in any given plan.
