# Supplementary material for: Reducing Human-Robot Goal State Divergence with Environment Design
Source: arXiv:2404.15184 source file (2024-04-10)
Supplement: Supplementary file 2 [file 5-1-needs-to-go-into-appendix.tex]

To calculate $\MxGDstr$ and $\MnGDstr$, we can place additional constraints on the human part of the plan to restrict plans of cost higher than the cost $C_{\epsilon}$. While in the most general case, this would involve additional book-keeping, one of the special cases, namely restricting to just optimal plans in the human model (represented as  $\MxGDOpt$ and $\MnGDOpt$) allows for a surprisingly simple formulation.
\begin{prop}
    For a given compiled model $\mathcal{\lambda}$, let us adopt the following cost function
    \begin{itemize}
        \item Cost of the human and robot action copies follows the ordering in the original models. For human action copies, this means, for any two actions $a_1,a_2 \in \mathcal{A^H_B}$,  $C^\lambda(a_1) < C^\lambda(a_2)$, if and only if, $C^\mathcal{H}(a_1^H) < C^\mathcal{H}(a_2^H)$, where $a_1,a_2 \in \mathcal{A^H}$ are the corresponding human actions. The same ordering constraint holds for $\mathcal{A^{R'}}$ and $\mathcal{A^R}$
        \item Cost of the cheapest human action is higher than the costs of the costliest robot plan, i.e., 
        $min_{a \in \mathcal{A^{H}_B}}(C^\lambda(a)) > max_{a \in \mathcal{A^{R'}}}(C^\lambda(a)) \times 2^{|\mathcal{F^R}|}$
        \item 
        Cost of the cheapest robot action is higher than the sum of the costs of all check agreement actions, i.e.
        $min_{a \in \mathcal{A^{R'}}}(C^\lambda(a)) > \sum_{f \in F} \mathcal{P}_1$
        
        \item Cost of check agreement action is unit cost (i.e. $\mathcal{P}_2 = 1$) and disagreement is $\mathcal{P}_2 = 0$.
    \end{itemize}
     For the given cost function, let $\pi$ be an optimal plan, then $\MxGDOpt(\mathcal{M}^R, \mathcal{M}^H) = |\kappa^-(\pi)|$.
\end{prop}
\begin{proof} [Proof Sketch]
    The cost function employed ensures that no optimal plan can contain a suboptimal human plan in it. Among all the solutions where $\mathcal{H}(\pi^{\lambda})$ corresponds to an optimal plan, the cost is dominated by  robot actions. 
    Thus no amount of agreement or disagreement would justify the selection of a suboptimal plan for  $\mathcal{R}(\pi^{\lambda})$. Finally, among the optimal robot and human plans, it selects ones that minimize the use of agreement actions.
\end{proof}

One can also calculate $\MnGDOpt$, by using a cost function that is pretty much the same as the one described above, except now $\mathcal{P}_1 =0$ and $\mathcal{P}_2 > 2^{|\mathcal{F^R}|}$.
